# Supplementary material for: Multi-Modal MPPI and Active Inference for Reactive Task and Motion Planning
Source: arXiv:2312.02328 source file (2024-07-10)
Supplement: Supplementary file 1 [file appendix-a.tex]

\section{Metric for measuring orientations}

It has been an essential issue to correctly represent 3D rotations and to efficiently evaluate the distance between them. \cite{huynh2009metrics} provided a detailed analysis of six metrics for measuring the distance between orientations, including Euclidean distance between the Euler angles, norm of the difference of quaternions, inner product of unit quaternions, and so on. However, these can not handle symmetric objects, which is challenging since different orientations may generate identical observations. \cite{xiang2017posecnn} introduced ShapeMatch-Loss to focus on matching the orientations for symmetric objects. Although it does not require the specification of symmetries, it is not efficient to compute for the fully symmetric objects, such as the cubes, as we will mainly use in the experiments to interact with.

% For non-symmetric objects, if we want to align these two orientations perfectly, it might be true to require the two quaternions or Euler angles to be exactly the same. However, this is not the case if we want to align the orientations of two fully symmetric objects, such as two cubes. This is due to the fact the flipping of the objects will lead to a different quaternion or Euler angle, but it may still have the same orientation as it is symmetric.

Therefore, we propose a new metric to efficiently evaluate two orientations for fully symmetric objects in a general way. We will first give the definition of general equivalence for fully symmetric objects. And then we will try to derive a proposition that meets the definition and prove it to be sufficient and necessary. Finally, we will show the proposed metric given the proved proposition.

\textbf{Definition 1} We say two three-dimensional Cartesian coordinates are in general equivalence if it holds that:
\begin{equation}
\label{eq:def1}
\begin{split}
    |\Vec{u}_1 \cdot \Vec{v}_i| &= 1, i \in \{1, 2, 3\} \\
    |\Vec{u}_2 \cdot \Vec{v}_j| &= 1, j \in \{1, 2, 3\} \\
    |\Vec{u}_3 \cdot \Vec{v}_k| &= 1, k \in \{1, 2, 3\} \\
\end{split}
\end{equation}
where $ i \neq j \neq k $, $\{\Vec{u}_1, \Vec{u}_2, \Vec{u}_3 \}$ and $\{\Vec{v}_1, \Vec{v}_2, \Vec{v}_3 \}$ form the orthogonal bases of the two coordinates respectively. 

\textbf{Proposition 1} There are two vectors (axes) in one coordinate that are collinear with some two vectors in another coordinate such that:
\begin{equation}
\begin{split}
    |\Vec{u}_m \cdot \Vec{v}_i| &= 1, m, i \in \{1, 2, 3\} \\
    |\Vec{u}_n \cdot \Vec{v}_j| &= 1, n, j \in \{1, 2, 3\} \\
\end{split}
\end{equation}
where $m \neq n,  i \neq j $. We will show that proposition 1 is equivalent to definition 1. 

\textbf{Theorem 1} Proposition 1 and definition 1 are equivalent. 
\begin{proof}
\hspace*{\fill}\\
\indent 1) We will first show proposition 1 is a sufficient condition of definition 1. We assume $\{\Vec{u}_m, \Vec{u}_n, \Vec{u}_p \}$ and $\{\Vec{v}_i, \Vec{v}_j, \Vec{v}_k \}$ form the orthogonal bases of the two coordinates respectively. If there are two vectors $\Vec{u}_m, \Vec{u}_n$ that are collinear with $\Vec{v}_i, \Vec{v}_j$, then $\Vec{u}_p$ is orthogonal to the plane these vectors span. So is $\Vec{v}_k$. Thus $\Vec{u}_p, \Vec{v}_k$ are collinear. Thus it meets \autoref{eq:def1} and thus meets definition 1.

2) Proposition 1 is also a necessary condition of definition 1. This is because if the two coordinates meet definition 1, there must be 4 vectors in the same plane. They are collinear.
\end{proof}


Theorem 1 allows us to simplify definition 1 and ignore a specific mapping between the vectors of coordinates, which would be difficult to find due to the flipping of cubes. Proposition 1 allows us to only focus on finding two pairs of collinear vectors in the two coordinates. Using this, we can derive our proposed metric to measure the difference in orientations of two symmetric objects.

\textbf{Metric}
\begin{equation}
\label{eq: ori_metric}
\begin{split}
    \phi(\Sigma_u, \Sigma_v) &= \min_{i, j \in \{1, 2, 3\}} 1 - |\Vec{u}_1 \cdot \Vec{v}_i| + 1 - |\Vec{u}_2 \cdot \Vec{v}_j| \\
     &= \min_{i, j \in \{1, 2, 3\}} 2 - |\Vec{u}_1 \cdot \Vec{v}_i| - |\Vec{u}_2 \cdot \Vec{v}_j| \\
\end{split}
\end{equation}
where $\Sigma_u = \{\Vec{u}_1, \Vec{u}_2, \Vec{u}_3 \}, \Sigma_v = \{\Vec{v}_1, \Vec{v}_2, \Vec{v}_3 \}$ form the orthogonal bases of two coordinates.

The major difference of our metric and ShapeMatch-Loss in \cite{xiang2017posecnn} is the simplification of only choosing two axes in one coordinate to match with the axes in another coordinate, which is supported by theorem 1.

% % The active inference algorithm for action selection is summarised in Algorithm \ref{alg:action_selection}. The algorithm starts by setting the prior preferences over observations. Then it enters the loop by getting observations and computing the VFE for each plan. The posterior state is then updated to compute the EFE for each plan. Once the terms of free energy are computed, we can obtain the posterior distribution over all possible plans and the overall probability distribution for the states. Finally, the action with the highest probability is selected among the possible plans.

% % \begin{algorithm}[H]
% %     \caption{Action selection with active inference \cite{pezzato2022aipbt}}\label{alg:action_selection}
% %     \begin{algorithmic}[1]
% %         \STATE Set $\boldsymbol{C}$                     \hfill $\triangleright$ Prior preferences
% %         \FOR {$\tau=1$ to $T$}
% %         \STATE If not specified, get state from $\boldsymbol{D}$ if $\tau == 1$
% %         \STATE If not specified, get observation from $\boldsymbol{A}$
% %         \STATE Compute $F$ for each plan                \hfill 
% %         \STATE Update posterior state $s_{\tau}^{\pi}$  \hfill 
% %         \STATE Compute $G$ for each plan                \hfill 
% %         \STATE Bayesian model averaging                 \hfill 
% %         \STATE Action selection                         \hfill 
% %         \ENDFOR
% %         \STATE \textbf{Return} $a$                      \hfill $\triangleright$ Preferred action
% %         \end{algorithmic}
% % \end{algorithm}

% The complete control scheme for adaptive action selection is shown in Algorithm \ref{alg:adaptive plans}.

% % The same as previous one
% % \begin{algorithm}[H]
% %     \caption{Generate adaptive plans with active inference \cite{pezzato2022aipbt}}\label{alg:adaptive plans}
% %     \begin{algorithmic}[1]
% %         \STATE /* \textit{Get desired prior and parameters from BT} */
% %         \STATE Set $\mathcal{C},$ param $\leftarrow $ BT                     \hfill $\triangleright$ With priority 1
% %         \STATE /* \textit{Set current observations, beliefs and logical state} */
% %         \STATE Set $\mathcal{O, S, L}_c(\tau)$
% %         \STATE /* \textit{Remove preferences with high-priority (i.e.} $>$ 1) \textit{if satisfied:}*/
% %         \FOR{all priors $\mathcal{C}^{(f_j)}$ with preference $\geq 1$}
% %             \IF{$l_c^{(f_j)}$ holds}
% %                 \STATE Remove pushed preference for $l_c^{(f_j)}$
% %             \ENDIF
% %         \ENDFOR
% %         \STATE /* \textit{Run active inference given} $\mathcal{O, S, C}$ */
% %         \STATE $a_\tau \leftarrow $ ActionSelection($\mathcal{O, S, C}$) \hfill $\triangleright$ Alg. \ref{alg:action_selection} 
% %         \STATE Update $\mathcal{L}_c(\tau)$
% %         \IF{$a_\tau$ == Idle}
% %             \STATE \textbf{return} Success \hfill $\triangleright$ No action required
% %         \ELSE 
% %             \STATE /* \textit{Check action preconditions} */
% %             \WHILE{$a_\tau$ != Idle}
% %                 \IF{ $prec_{a_\tau} \in \mathcal{L}_c(\tau)$ OR $prec_{a_\tau} = \emptyset$}
% %                     \STATE Execute($a_\tau$)
% %                     \STATE \textbf{break, return} Running \hfill $\triangleright$ Executing $a_\tau$
% %                 \ELSE
% %                     \STATE /* \textit{Push missing preconditions in} $\mathcal{C}$ */
% %                     \STATE $\mathcal{C} \leftarrow prec_{a_\tau}$ \hfill $\triangleright$ With priority 2
% %                     \STATE /* Exclude $a_\tau$ and re-run Alg.\ref{alg:action_selection} */
% %                     \STATE Remove($a_\tau$)
% %                     \STATE $a_\tau \leftarrow $ ActionSelection($\mathcal{O, S, C}$)
% %                     \IF{$a_\tau $ == Idle}
% %                         \STATE \textbf{return} Failure \hfill $\triangleright$ No solution
% %                     \ENDIF
% %                 \ENDIF
% %             \ENDWHILE
% %         \ENDIF
% %         \end{algorithmic}
% % \end{algorithm}

% % Newnew
% \begin{algorithm}[H]
%     \caption{Generate adaptive plans with active inference \cite{pezzato2022aipbt}}\label{alg:adaptive plans}
%     \begin{algorithmic}[1]
%         \STATE /* \textit{Get desired prior and parameters from BT} */
%         \STATE Set $\mathcal{C},$ param $\leftarrow $ BT                     \hfill $\triangleright$ With priority 1
%         \STATE /* \textit{Set current observations, beliefs and logical state} */
%         \STATE Set $\mathcal{O, S, L}_c(\tau)$
%         \STATE /* \textit{Create a list to store current action plans} */
%         % \STATE Set $\mathcal{A} \leftarrow \emptyset$
%         \STATE /* \textit{Remove preferences with high-priority (i.e.} $>$ 1) \textit{if satisfied:}*/
%         \FOR{all priors $\mathcal{C}^{(f_j)}$ with preference $\geq 1$}
%             \IF{$l_c^{(f_j)}$ holds}
%                 \STATE Remove pushed preference for $l_c^{(f_j)}$
%             \ENDIF
%         \ENDFOR
%         \STATE /* \textit{Run the loop until the IdleSuccess action is found */}
%         \WHILE{IdleSuccess $\notin \mathcal{A}$}
%             \STATE /* \textit{Run active inference given} $\mathcal{O, S, C}$ */
%             \STATE $a_\tau \leftarrow $ ActionSelection($\mathcal{O, S, C}$) \hfill $\triangleright$ Alg. \ref{alg:action_selection} 
%             \STATE Update $\mathcal{L}_c(\tau)$
%             \IF{No action found}
%                 \STATE \textbf{return} Failure \hfill $\triangleright$ No action found
%             \ELSE 
%                 \STATE /* \textit{Check action preconditions} */
%                 \IF{ $prec_{a_\tau} \in \mathcal{L}_c(\tau)$ OR $prec_{a_\tau} = \emptyset$}
%                     \STATE Execute($a_\tau$)
%                     \STATE $\mathcal{A}.append(a_\tau)$
%                     \STATE \textbf{break, return} Running \hfill $\triangleright$ Executing $a_\tau$
%                 \ELSE
%                     \STATE /* \textit{Push missing preconditions in} $\mathcal{C}$ */
%                     \STATE $\mathcal{C} \leftarrow prec_{a_\tau}$ \hfill $\triangleright$ With priority 2
%                     \STATE /* Exclude $a_\tau$ and re-run Alg.\ref{alg:action_selection} */
%                     \STATE Remove($a_\tau$)
%                     % \STATE $a_\tau \leftarrow $ ActionSelection($\mathcal{O, S, C}$)
%                     % \IF{$a_\tau $ == IdleSuccess}
%                     %     \STATE \textbf{return} Failure \hfill $\triangleright$ No solution
%                     % \ENDIF
%                 \ENDIF
%             \ENDIF
%         \ENDWHILE
%         % \STATE /* \textit{Create a list to store parallel plans} */
%         % \STATE Set $\mathcal{P} \leftarrow \emptyset$
%         % \STATE /* \textit{Parallelize current applicable actions} */
%         % \FOR{$a \in \mathcal{A}$}
%         %     \FOR{$b \in \mathcal{A}$}
%         %         \IF{$a \neq b$ \textbf{and} Parallelizable($a, b$)}
%         %             \STATE $\mathcal{P}.append([a, b])$
%         %         \ENDIF
%         %     \ENDFOR
%         % \ENDFOR
%         \STATE \textbf{Return} $\mathcal{A}$
%     \end{algorithmic}
% \end{algorithm}
